# Supplementary material for: Scan2Cap: Context-aware Dense Captioning in RGB-D Scans
Source: arXiv:2012.02206 source file (2020-12-03)
Supplement: Supplementary file 1 [file match_examples.tex]

\begin{figure}[!ht]
    \centering
%    \begin{subfigure}{\linewidth}
%        \centering
        \includegraphics[width=\linewidth]{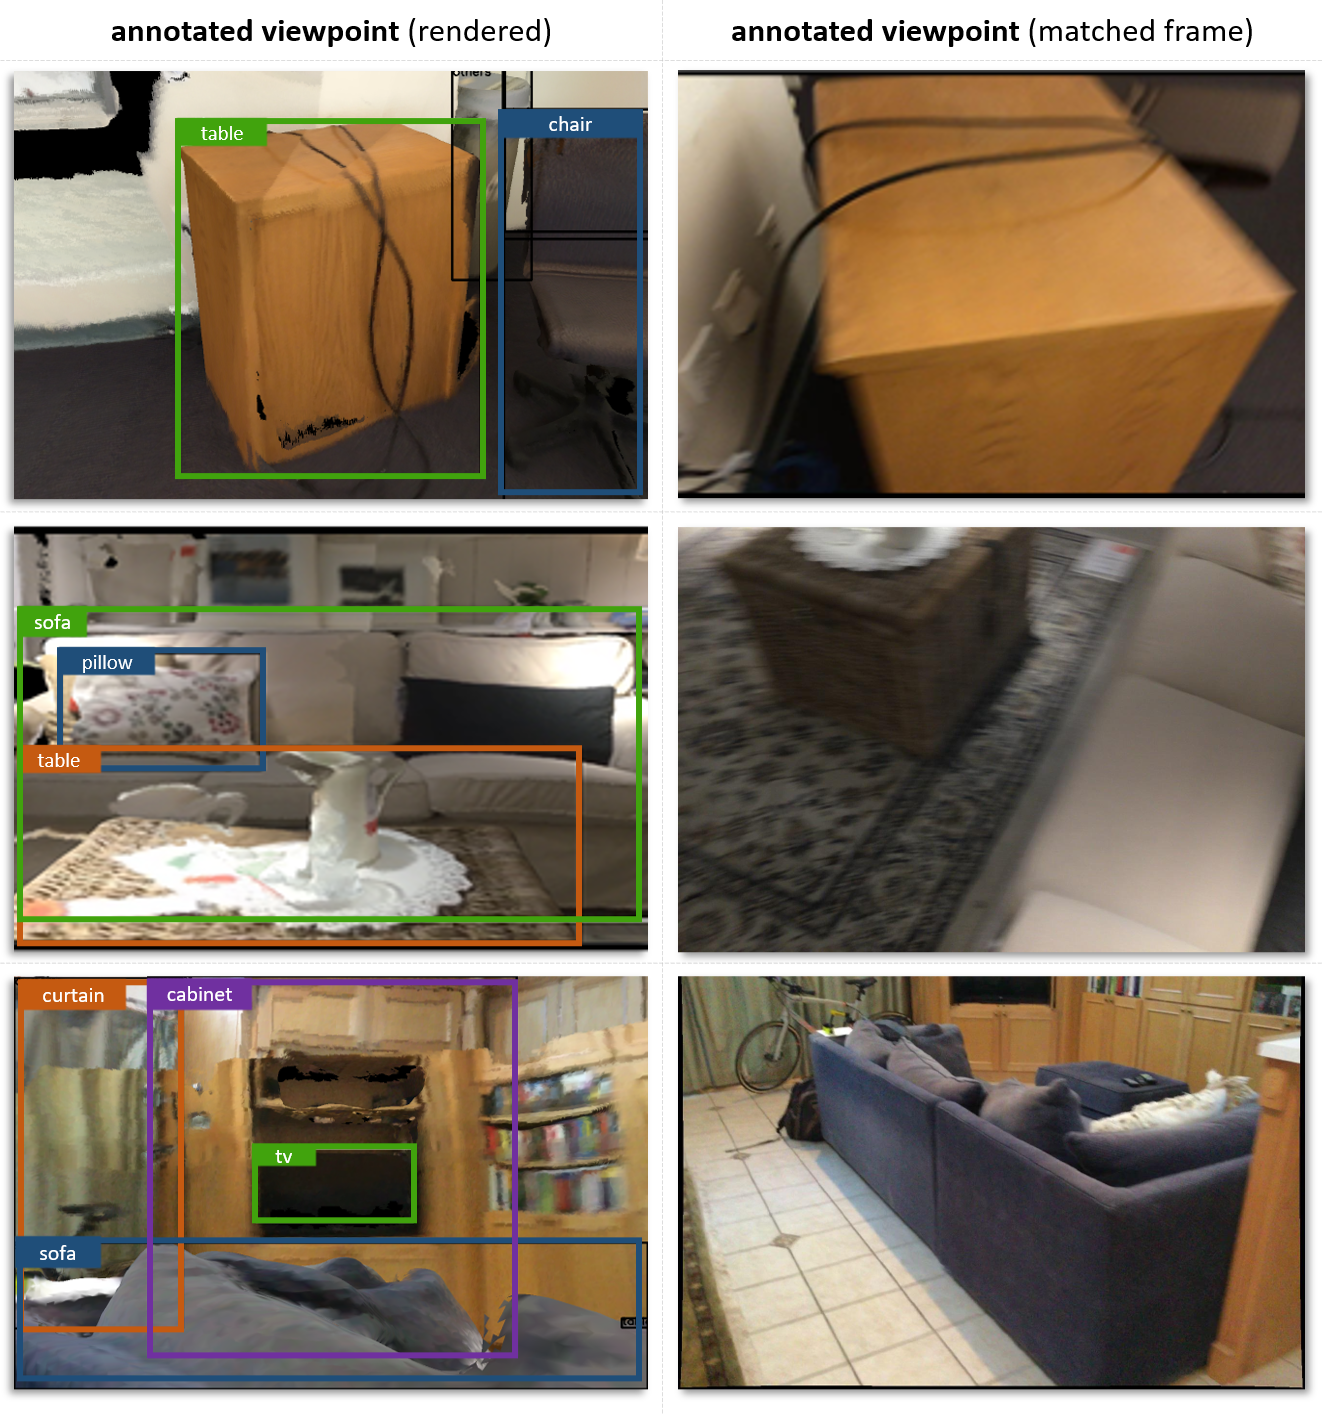}
        \caption{Examples of matched frames with 100\% target object existence accuracy. The target object is shown in green.}
        \label{fig:match_examples}
%        \end{subfigure}
    % \begin{subfigure}{\textwidth}
    %     \centering
    %     \includegraphics[width=0.99\linewidth]{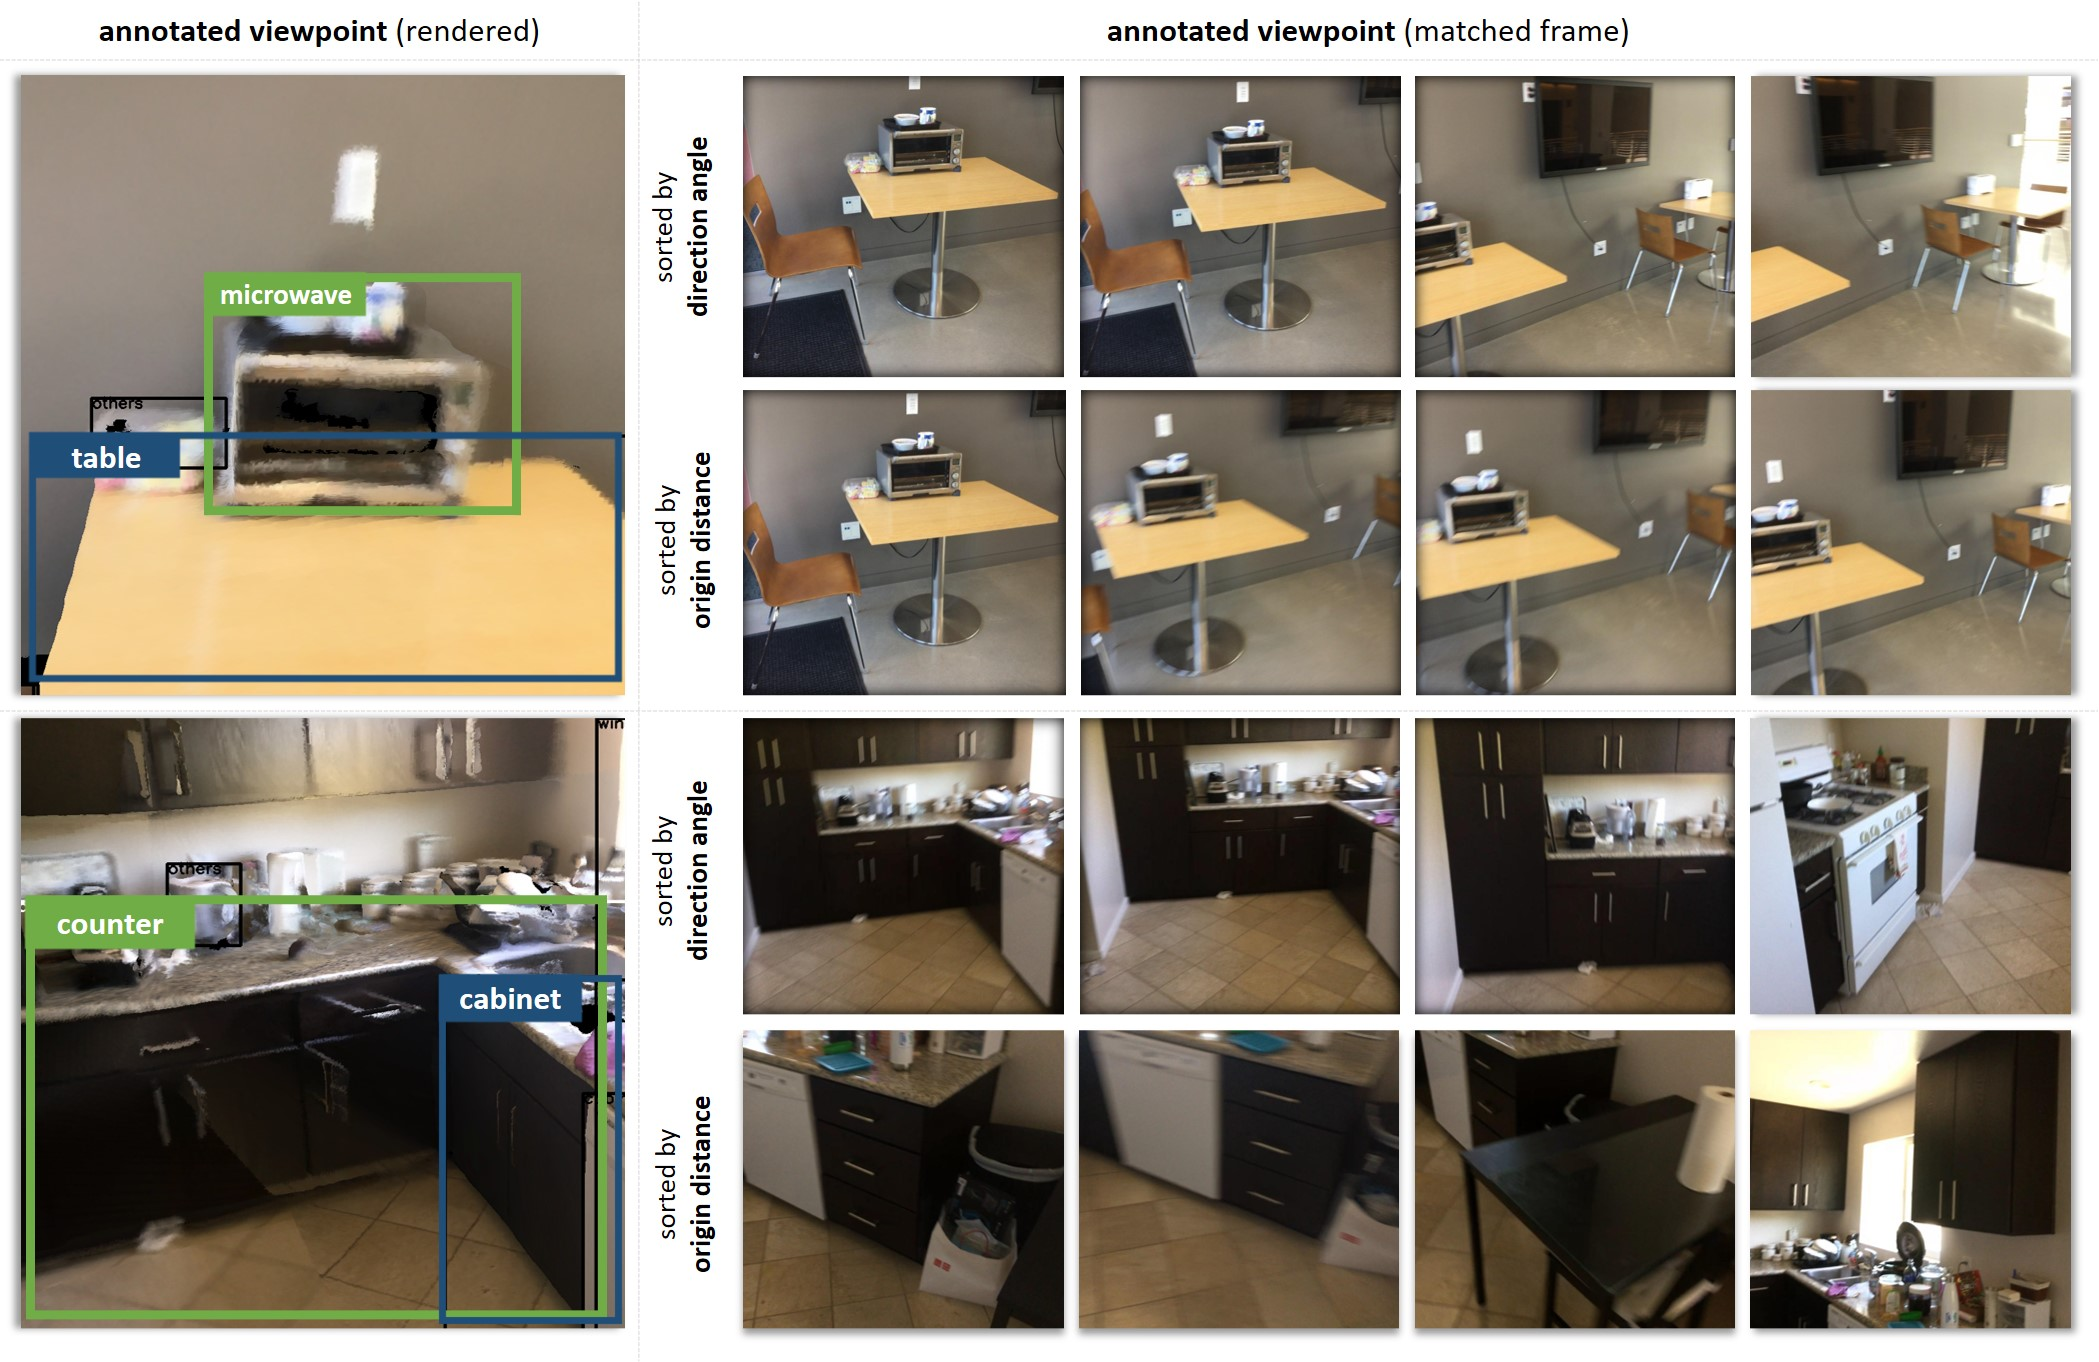}
    %     \caption{Examples of bad matched frames.}
    %     \label{fig:rendered_density}
    % \end{subfigure}
    % \caption{Examples of bad matches.}
    % \label{fig:modules}
\end{figure}
% \begin{figure*}[!ht]
%     \centering
%     \begin{subfigure}{\textwidth}
%         \centering
%         \includegraphics[width=\linewidth]{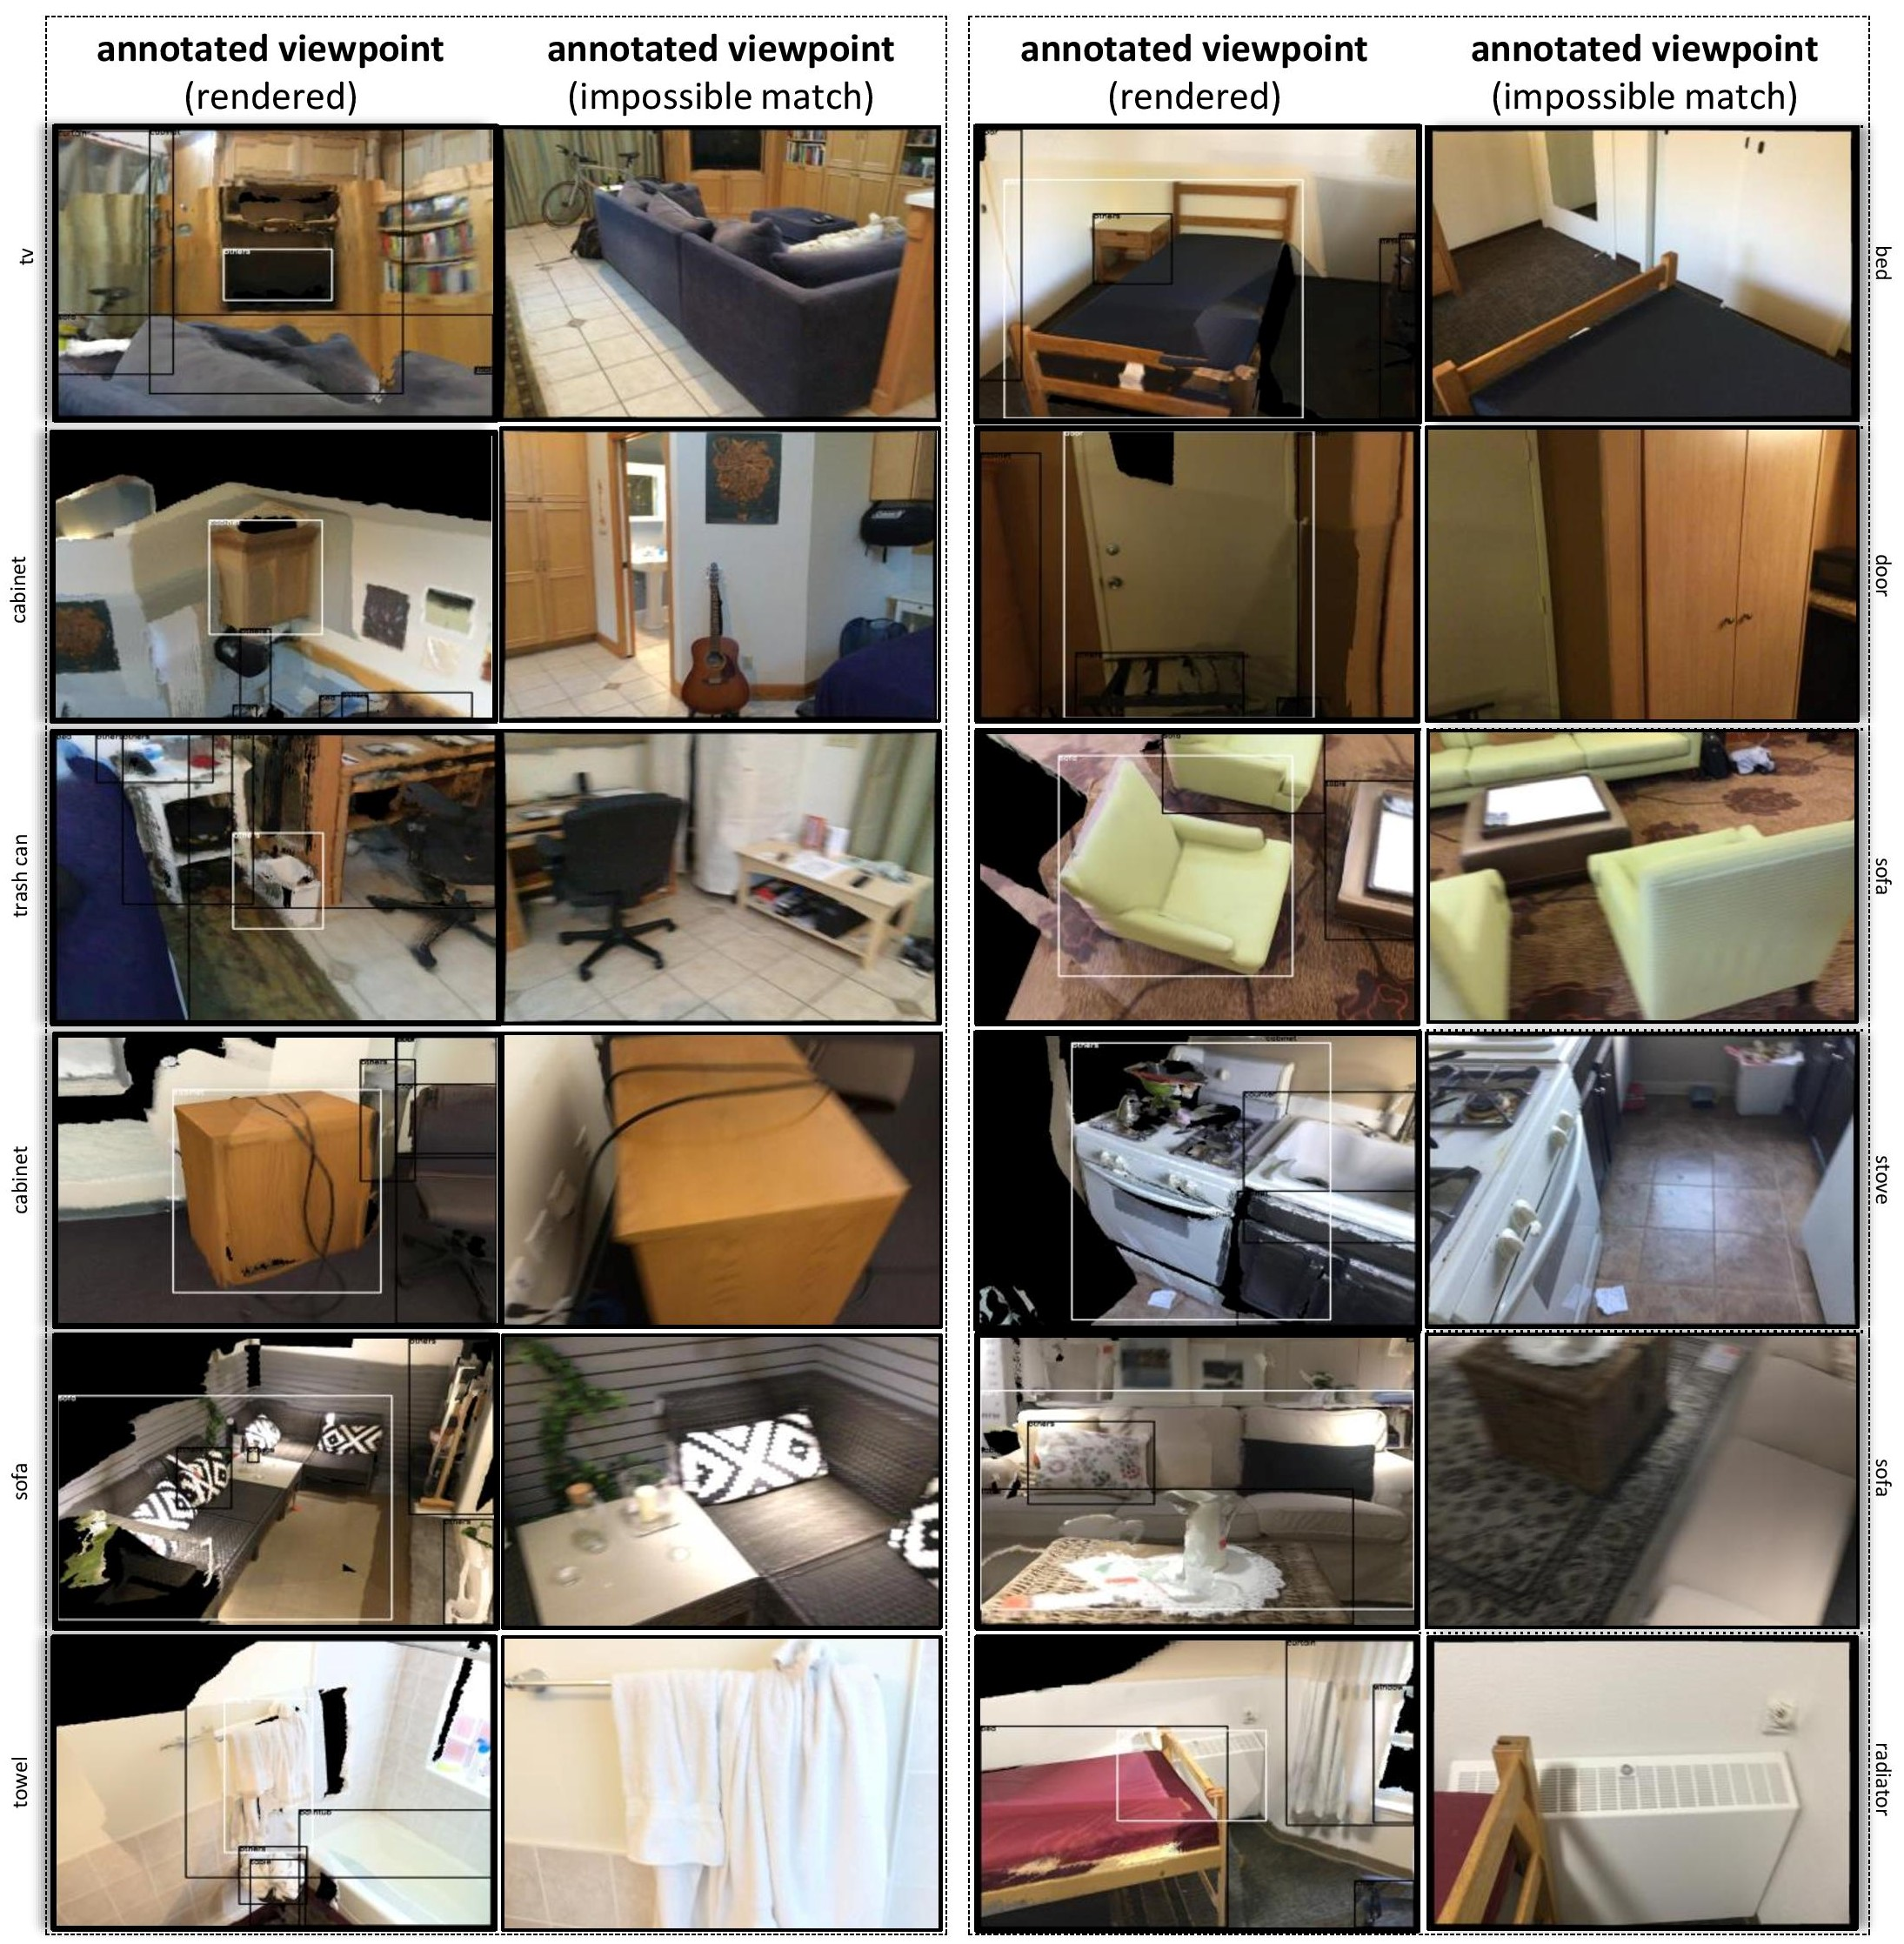}
%         \caption{Examples of impossible matches.}
%         \label{fig:rendered_object_ratio}
%         \end{subfigure}
%     % \begin{subfigure}{\textwidth}
%     %     \centering
%     %     \includegraphics[width=0.99\linewidth]{figures/supplements/sorted.jpg}
%     %     \caption{Examples of bad matched frames.}
%     %     \label{fig:rendered_density}
%     % \end{subfigure}
%     % \caption{Examples of bad matches.}
%     % \label{fig:modules}
% \end{figure*}
% \begin{figure*}[!ht]
%     \centering
%     \begin{subfigure}{\textwidth}
%         \centering
%         \includegraphics[width=\linewidth]{figures/supplements/sorted.jpg}
%         \caption{Matched viewpoints sorted by direction angle or origin distance.}
%         \label{fig:rendered_object_ratio}
%         \end{subfigure}
%     % \begin{subfigure}{\textwidth}
%     %     \centering
%     %     \includegraphics[width=0.99\linewidth]{figures/supplements/sorted.jpg}
%     %     \caption{Examples of bad matched frames.}
%     %     \label{fig:rendered_density}
%     % \end{subfigure}
%     % \caption{Examples of bad matches.}
%     % \label{fig:modules}
% \end{figure*}
