# Supplementary material for: Scan2Cap: Context-aware Dense Captioning in RGB-D Scans
Source: arXiv:2012.02206 source file (2020-12-03)
Supplement: Supplementary file 2 [file object_percentage.tex]

\begin{table}[t]
    \centering
    % \resizebox{\linewidth}{!}{
        %
        \begin{tabular}{l|cccc}
            \toprule
            & BEV & A+M & A+R & E \\
            \midrule
            Percentage & $99.93\%$ & $100\%$ & $99.68\%$ & $55.69\%$ \\
            \bottomrule
        \end{tabular}
        %
    % }
    \caption{Percentage of viewpoints that include the target object.}
    \label{tab:object_percentage}
\end{table}
