# Supplementary material for: Scan2Cap: Context-aware Dense Captioning in RGB-D Scans
Source: arXiv:2012.02206 source file (2020-12-03)
Supplement: Supplementary file 3 [file results_2dcap_match_based.tex]

\begin{table}[t]
    \centering
    \resizebox{\linewidth}{!}{
        \begin{tabular}{l|l|l|l|cccc}
            \toprule
            \multicolumn{8}{c}{Description Generation in 2D (Matched Frames)} \\
            \midrule
             VF & VP & DET & CAP & C & B-4 & M & R \\
            \midrule
            G  & A & - & S\&T & 11.5 & 1.63 & 5.64 & 13.86 \\ 
            G  + T  & A & O & S\&T  & \best{16.76} & \best{2.013} & \best{6.14} & 14.23 \\ 
            T  + C  & A & O & TD & 12.77 & 1.58 & 5.84 & \best{15.42} \\ 
            G  + T + C  & A & O & TD & 14 & 1.68 & 5.74 & 15.41 \\ 
            \bottomrule
        \end{tabular}
    }
    \caption{Results of caption generation with matched frames on the ScanRefer~\citep{chen2020scanrefer} validation split. Abbreviations are explained in Tab. \ref{tab:comp_baseline}.}
    \label{tab:match_baseline}
\end{table}
