# Supplementary material for: Scan2Cap: Context-aware Dense Captioning in RGB-D Scans
Source: arXiv:2012.02206 source file (2020-12-03)
Supplement: Supplementary file 4 [file results_2dcap_old.tex]

\begin{table*}[!ht]
    \centering
    \resizebox{\textwidth}{!}{
        %
        \begin{tabular}{l|l|l|l|cccc|l}
            \toprule
            \multicolumn{9}{c}{Description Generation in 2D (Rendered Viewpoints)} \\
            \midrule
             VF & VP & DET & CAP & C & B-4 & M & R & Prediction Example \\
            \midrule
            G  & A  & - & Retr &  12.07 & 4.58 &  11.5 &  29.37 & this is a white folding chair. it is at a black table. \\ 
            G  & A  & - & S\&T &  49.61 & 11.41 &  15.64 &  40.59 & this is a black chair. it is facing a desk. \\ 
            \midrule
            T  & A & O & Retr & 23 & 7.28 & 13.44 & 33.82 & there is a grey chair in front of a desk. there is a backpack sitting on the desk in front of it. \\ 
            T  + C  & A & O & TD & 51.35 & \best{13.09} & 15.88 & \best{43.52} & this is a brown chair. it is to the right of the table. \\ 
            T  + C  & A & O & M$^2$ & 34.72 & 7.13 & 12.69 & 33.6 & this is a black chair it is at a desk. \\ 
            T  + C  & A & O & M$^2$ RL & 42.77 & 9.03 & 14.34 & 36.27 & this is a black office chair it is in front of the desk. \\ 
            G  + T  & A & O & S\&T &  \best{59.12} & 12.73 & \best{16.61} & 41.32 & this is a black chair. it is facing a desk. \\ 
             G  + T + C  & A & O & TD &  18.1 & 5.65 & 11.37 & 33.1 & this chair is facing the. it is is is. \\ 
            \midrule
            T  + C   & A & 2DM & TD & 35.65 & \best{11} & 14.3 & \best{40.7} & this is a black chair. it is in the corner. \\ 
            T  + C   & A & 2DM & M$^2$ & 31.02 & 7.19 &  12.28 &  33.22 & this is a black chair it is at a desk. \\
            T  + C   & A & 2DM & M$^2$ RL & 35.91 & 8.52 &  13.53 &  35.33 & this is a black chair it is to the right of the chair. \\ 
            G  + T  & A & 2DM & S\&T &  \best{41.44} & 10.95 &  \best{15.08} &  39.04 & this is a black monitor. it is on a desk.  \\ 
            G  + T + C  & A & 2DM & TD &  14.84 & 4.95 &  10.85 &  31.52 & this is a black chair chair. is is the the. \\ 
            \midrule
            G  & E  & - & S\&T &  28.52 & 24.03 &  18.92 &  47.76 & this is a black chair. it is facing a table. \\ 
            T  + C  & E &  3DV & TD & 28.25 & \best{30.11} &  18.9 &  \best{52.14} & this is a black tv. it is on the wall. \\ 
            T  + C  & E &  3DV & M$^2$ & 11.44 & 19.67 &  14.23 &  40.42 & this is a black chair, it is to the right of another chair. \\ 
            T  + C  & E &  3DV & M$^2$ RL & 11.83 & 24.79 &  15.47 &  42.69 & this is a black chair, it is to the right of the table. \\ 
            G  + T  & E & 3DV & S\&T &  \best{31.48} & 25.35 &  \best{19.09} &  47.06 & this chair is in the middle. it is facing left. \\ 
            G  + T + C  & E &  3DV & TD & 9.66 & 9.68 &  13.14 &  38.38 & this is a black tv. it is on the wall.\\ 
%            \midrule
%            G & BEV & - & S\&T & 19.94 & 8.74 & \best{14.64} & 36.53 & the chair is black and is sitting in front of the desk. it is to the right of the chair. \\
%            G + T & BEV & O & S\&T & \best{24.21} & \best{9.69} & 14.41 & \best{37.38} & the chair is black and is pushed into the table. it is to the right of the chair. \\
            \bottomrule
        \end{tabular}
        %
    }
    \caption{Results of caption generation with rendered viewpoints on the ScanRefer~\citep{chen2020scanrefer} validation split. Metrics are calculated using the one-to-one evalution approach. \textbf{VF} is the input visual feature which can include the full image (G), context object (C), and/or target object (T). \textbf{VP} is the viewpoint that can be annotated (A), estimated (E), or bird's eye viewpoint (BEV). \textbf{DET} is the object bounding box which can be the ground truth box (O), Mask R-CNN~\citep{he2017mask} detected in 2D (2DM) or back-projected VoteNet~\citep{qi2019deep} detection in 3D (3DV). \textbf{CAP} is the captioning method which can be cosine retrieval (Retr), Show and tell (S\&T)~\citep{vinyals2015show}, Top-down attention~\citep{anderson2018bottom} (TD), Meshed memory transformer~\citep{cornia2020meshed} without and with self-critical optimization repsectively (M$^2$) and (M$^2$ RL). Rendered viewpoints for the prediction example are provided in Fig.~\ref{fig:qualitative_2d}.}
    \label{tab:comp_baseline}
\end{table*}
